# Supplementary material for: Annolid: Annotate, Segment, and Track Anything You Need
Source: arXiv:2403.18690 source file (2024-03-27)
Supplement: Supplementary file 1 [file 09-appendix.tex]

% \appendix
% \beginsupplement
\onecolumn

% Moved the Related Works section here as 'supplementary data'
\section{Related Works}

\paragraph{Tracking-by-Detection Approaches.}

Tracking-by-detection methodologies, as highlighted in studies such as \cite{kim2015multiple,tang2017multiple,bergmann2019tracking}, conventionally hinge upon the detection of segmentations within each frame, subsequently employing temporal propagation to link these per-frame segmentations. Notably, pose estimation-based multi-animal tracking packages like those elucidated in \cite{Lauer2022MultianimalPE,Pereira2022sleap} have garnered popularity. These solutions necessitate the labeling and training of networks to estimate poses, followed by the utilization of various techniques to identify and associate instances across frames. Moreover, these tools equip users with functionalities for manual correction and track merging, thereby enhancing the robustness and accuracy of the tracking process.

\paragraph{Universal Segmentation Tracking and Decoupled Video Segmentation.}

In the realm of video object segmentation, conventional 'tracking-by-detection' methods hinge on image-level detections and short-term temporal tracking. However, recent advancements like SAM-PT \cite{rajivc2023segment} and DEVA \cite{cheng2023tracking} have introduced innovative strategies. The Segment Anything (SAM) framework, as demonstrated by Kirillov et al. \cite{kirillov2023segment}, underscores the efficacy and adaptability of large-scale training for universal image segmentation, thereby laying significant groundwork for open-world segmentation. Subsequent studies by Yang et al. \cite{yang2023track} and Cheng et al. \cite{cheng2023segment} extend SAM to video data by propagating masks generated by SAM using video object segmentation algorithms. Nevertheless, these approaches predominantly rely on single-frame segmentation and lack inherent denoising capability. To address this limitation, Cheng et al. \cite{cheng2023tracking} proposed an in-clip consensus approach.

\paragraph{Tracking by classifing Segmentation Masks.}

idTracker.ai \cite{romero2019idtracker} employs threshold-based segmentation to isolate instances within frames, followed by classification networks to identify individual animals. Annolid \cite{yang2023automated} utilizes instance segmentation networks such as Mask R-CNN for segmentation and classification by assigning each instance its own class. SIPEC \cite{marks2022deep} utilizes an instance segmentation network to delineate animals within video frames and subsequently employs another network for animal identification, enabling the analysis of animal behavior in intricate environments using raw video data. SIPEC comprises four key modules: segmentation, identification, pose estimation, and behavioral classification. Notably, ~\cite{romero2019idtracker,marks2022deep} require more than 1000 labeled frames for training the identification networks.

\paragraph{Memory-Based VOS.}

Semi-supervised Video Object Segmentation (VOS) involves directional propagation of information, leading many existing approaches to employ a feature memory representation for storing past features to segment future frames. This includes online learning methods that finetune a network on the first-frame segmentation for each video during inference. XMem~\cite{cheng2022xmem} leverages various memory types to enhance performance and efficiency, albeit facing challenges from noise introduced by low-level pixel matching. Cutie integrates memory reading techniques inspired by XMem~\cite{cheng2022xmem} and introduces an object reading mechanism. This integration empowers Cutie to achieve superior performance, particularly in demanding scenarios.

\paragraph{End-to-End Video Segmentation.}

In the realm of semi-supervised Video Object Segmentation (VOS), the utilization of memory-based representations and Transformer-based methods has become pivotal for effectively segmenting future frames and conducting pixel matching with memory. A notable contribution in this domain is the introduction of Cutie~\cite{cheng2023putting}. Cutie presents an efficient object transformer framework that facilitates real-time processing by circumventing costly attention mechanisms. What sets Cutie apart is its ability to establish bi-directional communication between pixel-level and object-level features, thereby enhancing object-level reasoning. Unlike previous methods such as ISVOS~\cite{wang2023look}, Cutie adopts a fully-online approach that seamlessly segments subsequent frames within a video sequence. The bi-directional propagation mechanism used by Cutie unifies image segmentation and propagation models, enhancing video segmentation performance.One of the key strengths of Cutie lies in its integration of pixel memory and object memory representations, which enables the efficient retrieval and utilization of relevant information during segmentation tasks. Moreover, the incorporation of an object transformer enriches pixel features with object-level semantics, ensuring robust segmentation performance even in complex scenarios. Furthermore, Cutie's commitment to open-source principles enhances reproducibility and invites community contributions, thereby fostering collaborative advancements in the field of video object segmentation. Through its innovative design and practical implementation, Cutie represents a significant stride forward in the quest for efficient and effective video segmentation techniques.

\paragraph{Open-World Video Segmentation.}

Recently, the introduction of a novel open-world video segmentation dataset, BURST \cite{athar2023burst}, marks a notable advancement in the field. BURST encompasses 482 object classes across diverse scenarios, evaluating open-world performance through separate metric computations for common classes (78, overlapping with COCO) and uncommon classes (404). The baseline method in BURST \cite{athar2023burst} predicts object proposals via an image instance segmentation model trained on COCO \cite{lin2014microsoft}, associating these proposals frame-by-frame using either box IoU or STCN \cite{cheng2021stcn}. OWTB \cite{liu2022opening} extends this by incorporating optical flow and pre-trained Re-ID features for proposal association. In contrast, Cutie approaches utilizes bi-directional propagation to generate segmentations, minimizing sensitivity to image segmentation errors. Another significant open-world video segmentation dataset, UVO \cite{du2021uvo}, predominantly focuses on human actions. These refined distinctions among approaches and datasets illuminate the nuances of video object segmentation and its diverse applications.
